# Supplementary material for: Dueling Network Architectures for Deep Reinforcement Learning
Source: arXiv:1511.06581 source file (2016-04-05)
Supplement: Supplementary file 1 [file appendix.tex]

%!TEX root = main.tex
\label{sec:appen}
\begin{table}[!b]
\footnotesize
\caption{Raw scores across all games. Starting with {\bf 30 no-op} actions.}
\begin{center}
\begin{tabular}{l|rrr|rrr|rr}
{\sc Games} &  {\sc No. Actions} &     {\sc Random} &     {\sc Human} &        {\sc DQN} &       {\sc DDQN} &       {\sc Duel} &{\sc Prior.} & {\sc Prior. Duel.}\\
\hline
               Alien &              18 &      227.8 &   7,127.7 &    1,620.0 &    3,747.7 &{\bf4,461.4}&    4,203.8 &      3,941.0 \\
              Amidar &              10 &        5.8 &   1,719.5 &      978.0 &    1,793.3 &{\bf2,354.5}&    1,838.9 &      2,296.8 \\
             Assault &               7 &      222.4 &     742.0 &    4,280.4 &    5,393.2 &    4,621.0 &    7,672.1 &{\bf11,477.0}\\
             Asterix &               9 &      210.0 &   8,503.3 &    4,359.0 &   17,356.5 &   28,188.0 &   31,527.0 &{\bf375,080.0}\\
           Asteroids &              14 &      719.1 &  47,388.7 &    1,364.5 &      734.7 &{\bf2,837.7}&    2,654.3 &      1,192.7 \\
            Atlantis &               4 &   12,850.0 &  29,028.1 &  279,987.0 &  106,056.0 &  382,572.0 &  357,324.0 &{\bf395,762.0}\\
          Bank Heist &              18 &       14.2 &     753.1 &      455.0 &    1,030.6 &{\bf1,611.9}&    1,054.6 &      1,503.1 \\
         Battle Zone &              18 &    2,360.0 &  37,187.5 &   29,900.0 &   31,700.0 &{\bf37,150.0}&   31,530.0 &     35,520.0 \\
          Beam Rider &               9 &      363.9 &  16,926.5 &    8,627.5 &   13,772.8 &   12,164.0 &   23,384.2 &{\bf30,276.5}\\
             Berzerk &              18 &      123.7 &   2,630.4 &      585.6 &    1,225.4 &    1,472.6 &    1,305.6 &{\bf3,409.0}\\
             Bowling &               6 &       23.1 &     160.7 &       50.4 &{\bf68.1}&       65.5 &       47.9 &         46.7 \\
              Boxing &              18 &        0.1 &      12.1 &       88.0 &       91.6 &{\bf99.4}&       95.6 &         98.9 \\
            Breakout &               4 &        1.7 &      30.5 &      385.5 &{\bf418.5}&      345.3 &      373.9 &        366.0 \\
           Centipede &              18 &    2,090.9 &  12,017.0 &    4,657.7 &    5,409.4 &    7,561.4 &    4,463.2 &{\bf7,687.5}\\
     Chopper Command &              18 &      811.0 &   7,387.8 &    6,126.0 &    5,809.0 &   11,215.0 &    8,600.0 &{\bf13,185.0}\\
       Crazy Climber &               9 &   10,780.5 &  35,829.4 &  110,763.0 &  117,282.0 &  143,570.0 &  141,161.0 &{\bf162,224.0}\\
            Defender &              18 &    2,874.5 &  18,688.9 &   23,633.0 &   35,338.5 &{\bf42,214.0}&   31,286.5 &     41,324.5 \\
        Demon Attack &               6 &      152.1 &   1,971.0 &   12,149.4 &   58,044.2 &   60,813.3 &   71,846.4 &{\bf72,878.6}\\
         Double Dunk &              18 &      -18.6 &     -16.4 &       -6.6 &       -5.5 &        0.1 &{\bf18.5}&        -12.5 \\
              Enduro &               9 &        0.0 &     860.5 &      729.0 &    1,211.8 &    2,258.2 &    2,093.0 &{\bf2,306.4}\\
       Fishing Derby &              18 &      -91.7 &     -38.7 &       -4.9 &       15.5 &{\bf46.4}&       39.5 &         41.3 \\
             Freeway &               3 &        0.0 &      29.6 &       30.8 &       33.3 &        0.0 &{\bf33.7}&         33.0 \\
           Frostbite &              18 &       65.2 &   4,334.7 &      797.4 &    1,683.3 &    4,672.8 &    4,380.1 &{\bf7,413.0}\\
              Gopher &               8 &      257.6 &   2,412.5 &    8,777.4 &   14,840.8 &   15,718.4 &   32,487.2 &{\bf104,368.2}\\
            Gravitar &              18 &      173.0 &   3,351.4 &      473.0 &      412.0 &{\bf588.0}&      548.5 &        238.0 \\
            H.E.R.O. &              18 &    1,027.0 &  30,826.4 &   20,437.8 &   20,130.2 &   20,818.2 &{\bf23,037.7}&     21,036.5 \\
          Ice Hockey &              18 &      -11.2 &       0.9 &       -1.9 &       -2.7 &        0.5 &{\bf1.3}&         -0.4 \\
          James Bond &              18 &       29.0 &     302.8 &      768.5 &    1,358.0 &    1,312.5 &{\bf5,148.0}&        812.0 \\
            Kangaroo &              18 &       52.0 &   3,035.0 &    7,259.0 &   12,992.0 &   14,854.0 &{\bf16,200.0}&      1,792.0 \\
               Krull &              18 &    1,598.0 &   2,665.5 &    8,422.3 &    7,920.5 &{\bf11,451.9}&    9,728.0 &     10,374.4 \\
      Kung-Fu Master &              14 &      258.5 &  22,736.3 &   26,059.0 &   29,710.0 &   34,294.0 &   39,581.0 &{\bf48,375.0}\\
 Montezuma's Revenge &              18 &        0.0 &   4,753.3 &{\bf0.0}&        0.0 &        0.0 &        0.0 &          0.0 \\
         Ms. Pac-Man &               9 &      307.3 &   6,951.6 &    3,085.6 &    2,711.4 &    6,283.5 &{\bf6,518.7}&      3,327.3 \\
      Name This Game &               6 &    2,292.3 &   8,049.0 &    8,207.8 &   10,616.0 &   11,971.1 &   12,270.5 &{\bf15,572.5}\\
             Phoenix &               8 &      761.4 &   7,242.6 &    8,485.2 &   12,252.5 &   23,092.2 &   18,992.7 &{\bf70,324.3}\\
            Pitfall! &              18 &     -229.4 &   6,463.7 &     -286.1 &      -29.9 &{\bf0.0}&     -356.5 &          0.0 \\
                Pong &               3 &      -20.7 &      14.6 &       19.5 &       20.9 &{\bf21.0}&       20.6 &         20.9 \\
         Private Eye &              18 &       24.9 &  69,571.3 &      146.7 &      129.7 &      103.0 &      200.0 &{\bf206.0}\\
              Q*Bert &               6 &      163.9 &  13,455.0 &   13,117.3 &   15,088.5 &{\bf19,220.3}&   16,256.5 &     18,760.3 \\
          River Raid &              18 &    1,338.5 &  17,118.0 &    7,377.6 &   14,884.5 &{\bf21,162.6}&   14,522.3 &     20,607.6 \\
         Road Runner &              18 &       11.5 &   7,845.0 &   39,544.0 &   44,127.0 &{\bf69,524.0}&   57,608.0 &     62,151.0 \\
            Robotank &              18 &        2.2 &      11.9 &       63.9 &       65.1 &{\bf65.3}&       62.6 &         27.5 \\
            Seaquest &              18 &       68.4 &  42,054.7 &    5,860.6 &   16,452.7 &{\bf50,254.2}&   26,357.8 &        931.6 \\
              Skiing &               3 &  -17,098.1 &  -4,336.9 &  -13,062.3 &   -9,021.8 &{\bf-8,857.4}&   -9,996.9 &    -19,949.9 \\
             Solaris &              18 &    1,236.3 &  12,326.7 &    3,482.8 &    3,067.8 &    2,250.8 &{\bf4,309.0}&        133.4 \\
      Space Invaders &               6 &      148.0 &   1,668.7 &    1,692.3 &    2,525.5 &    6,427.3 &    2,865.8 &{\bf15,311.5}\\
         Star Gunner &              18 &      664.0 &  10,250.0 &   54,282.0 &   60,142.0 &   89,238.0 &   63,302.0 &{\bf125,117.0}\\
           Surround  &               5 &      -10.0 &       6.5 &       -5.6 &       -2.9 &        4.4 &{\bf8.9}&          1.2 \\
              Tennis &              18 &      -23.8 &      -8.3 &{\bf12.2}&      -22.8 &        5.1 &        0.0 &          0.0 \\
          Time Pilot &              10 &    3,568.0 &   5,229.2 &    4,870.0 &    8,339.0 &{\bf11,666.0}&    9,197.0 &      7,553.0 \\
           Tutankham &               8 &       11.4 &     167.6 &       68.1 &      218.4 &      211.4 &      204.6 &{\bf245.9}\\
         Up and Down &               6 &      533.4 &  11,693.2 &    9,989.9 &   22,972.2 &{\bf44,939.6}&   16,154.1 &     33,879.1 \\
             Venture &              18 &        0.0 &   1,187.5 &      163.0 &       98.0 &{\bf497.0}&       54.0 &         48.0 \\
       Video Pinball &               9 &   16,256.9 &  17,667.9 &  196,760.4 &  309,941.9 &   98,209.5 &  282,007.3 &{\bf479,197.0}\\
       Wizard Of Wor &              10 &      563.5 &   4,756.5 &    2,704.0 &    7,492.0 &    7,855.0 &    4,802.0 &{\bf12,352.0}\\
       Yars' Revenge &              18 &    3,092.9 &  54,576.9 &   18,098.9 &   11,712.6 &   49,622.1 &   11,357.0 &{\bf69,618.1}\\
              Zaxxon &              18 &       32.5 &   9,173.3 &    5,363.0 &   10,163.0 &   12,944.0 &   10,469.0 &{\bf13,886.0}\\
\end{tabular}
\end{center}
\end{table}

\begin{table}[t]
\caption{Raw scores across all games. Starting with {\bf Human starts}.}
\footnotesize
\begin{center}
\begin{tabular}{l|rrr|rrr|rr}
    {\sc Games} &  {\sc No. Actions} &     {\sc Random} &     {\sc Human} &        {\sc DQN} &       {\sc DDQN} &       {\sc Duel} &{\sc Prior.} & {\sc Prior. Duel.}\\
\hline
               Alien &              18 &      128.3 &   6,371.3 &      634.0 &    1,033.4 &{\bf1,486.5}&    1,334.7 &        823.7 \\
              Amidar &              10 &       11.8 &   1,540.4 &      178.4 &      169.1 &      172.7 &      129.1 &{\bf238.4}\\
             Assault &               7 &      166.9 &     628.9 &    3,489.3 &    6,060.8 &    3,994.8 &    6,548.9 &{\bf10,950.6}\\
             Asterix &               9 &      164.5 &   7,536.0 &    3,170.5 &   16,837.0 &   15,840.0 &   22,484.5 &{\bf364,200.0}\\
           Asteroids &              14 &      871.3 &  36,517.3 &    1,458.7 &    1,193.2 &{\bf2,035.4}&    1,745.1 &      1,021.9 \\
            Atlantis &               4 &   13,463.0 &  26,575.0 &  292,491.0 &  319,688.0 &{\bf445,360.0}&  330,647.0 &    423,252.0 \\
          Bank Heist &              18 &       21.7 &     644.5 &      312.7 &      886.0 &{\bf1,129.3}&      876.6 &      1,004.6 \\
         Battle Zone &              18 &    3,560.0 &  33,030.0 &   23,750.0 &   24,740.0 &{\bf31,320.0}&   25,520.0 &     30,650.0 \\
          Beam Rider &               9 &      254.6 &  14,961.0 &    9,743.2 &   17,417.2 &   14,591.3 &   31,181.3 &{\bf37,412.2}\\
             Berzerk &              18 &      196.1 &   2,237.5 &      493.4 &    1,011.1 &      910.6 &      865.9 &{\bf2,178.6}\\
             Bowling &               6 &       35.2 &     146.5 &       56.5 &{\bf69.6}&       65.7 &       52.0 &         50.4 \\
              Boxing &              18 &       -1.5 &       9.6 &       70.3 &       73.5 &       77.3 &       72.3 &{\bf79.2}\\
            Breakout &               4 &        1.6 &      27.9 &      354.5 &      368.9 &{\bf411.6}&      343.0 &        354.6 \\
           Centipede &              18 &    1,925.5 &  10,321.9 &    3,973.9 &    3,853.5 &    4,881.0 &    3,489.1 &{\bf5,570.2}\\
     Chopper Command &              18 &      644.0 &   8,930.0 &    5,017.0 &    3,495.0 &    3,784.0 &    4,635.0 &{\bf8,058.0}\\
       Crazy Climber &               9 &    9,337.0 &  32,667.0 &   98,128.0 &  113,782.0 &  124,566.0 &  127,512.0 &{\bf127,853.0}\\
            Defender &              18 &    1,965.5 &  14,296.0 &   15,917.5 &   27,510.0 &   33,996.0 &   23,666.5 &{\bf34,415.0}\\
        Demon Attack &               6 &      208.3 &   3,442.8 &   12,550.7 &   69,803.4 &   56,322.8 &   61,277.5 &{\bf73,371.3}\\
         Double Dunk &              18 &      -16.0 &     -14.4 &       -6.0 &       -0.3 &       -0.8 &{\bf16.0}&        -10.7 \\
              Enduro &               9 &      -81.8 &     740.2 &      626.7 &    1,216.6 &    2,077.4 &    1,831.0 &{\bf2,223.9}\\
       Fishing Derby &              18 &      -77.1 &       5.1 &       -1.6 &        3.2 &       -4.1 &        9.8 &{\bf17.0}\\
             Freeway &               3 &        0.1 &      25.6 &       26.9 &       28.8 &        0.2 &{\bf28.9}&         28.2 \\
           Frostbite &              18 &       66.4 &   4,202.8 &      496.1 &    1,448.1 &    2,332.4 &    3,510.0 &{\bf4,038.4}\\
              Gopher &               8 &      250.0 &   2,311.0 &    8,190.4 &   15,253.0 &   20,051.4 &   34,858.8 &{\bf105,148.4}\\
            Gravitar &              18 &      245.5 &   3,116.0 &{\bf298.0}&      200.5 &      297.0 &      269.5 &        167.0 \\
            H.E.R.O. &              18 &    1,580.3 &  25,839.4 &   14,992.9 &   14,892.5 &   15,207.9 &{\bf20,889.9}&     15,459.2 \\
          Ice Hockey &              18 &       -9.7 &       0.5 &       -1.6 &       -2.5 &       -1.3 &       -0.2 &{\bf0.5}\\
          James Bond &              18 &       33.5 &     368.5 &      697.5 &      573.0 &      835.5 &{\bf3,961.0}&        585.0 \\
            Kangaroo &              18 &      100.0 &   2,739.0 &    4,496.0 &   11,204.0 &   10,334.0 &{\bf12,185.0}&        861.0 \\
               Krull &              18 &    1,151.9 &   2,109.1 &    6,206.0 &    6,796.1 &{\bf8,051.6}&    6,872.8 &      7,658.6 \\
      Kung-Fu Master &              14 &      304.0 &  20,786.8 &   20,882.0 &   30,207.0 &   24,288.0 &   31,676.0 &{\bf37,484.0}\\
 Montezuma's Revenge &              18 &       25.0 &   4,182.0 &       47.0 &       42.0 &       22.0 &{\bf51.0}&         24.0 \\
         Ms. Pac-Man &               9 &      197.8 &  15,375.0 &    1,092.3 &    1,241.3 &{\bf2,250.6}&    1,865.9 &      1,007.8 \\
      Name This Game &               6 &    1,747.8 &   6,796.0 &    6,738.8 &    8,960.3 &   11,185.1 &   10,497.6 &{\bf13,637.9}\\
             Phoenix &               8 &    1,134.4 &   6,686.2 &    7,484.8 &   12,366.5 &   20,410.5 &   16,903.6 &{\bf63,597.0}\\
            Pitfall! &              18 &     -348.8 &   5,998.9 &     -113.2 &     -186.7 &{\bf-46.9}&     -427.0 &       -243.6 \\
                Pong &               3 &      -18.0 &      15.5 &       18.0 &{\bf19.1}&       18.8 &       18.9 &         18.4 \\
         Private Eye &              18 &      662.8 &  64,169.1 &      207.9 &     -575.5 &      292.6 &      670.7 &{\bf1,277.6}\\
              Q*Bert &               6 &      183.0 &  12,085.0 &    9,271.5 &   11,020.8 &{\bf14,175.8}&    9,944.0 &     14,063.0 \\
          River Raid &              18 &      588.3 &  14,382.2 &    4,748.5 &   10,838.4 &{\bf16,569.4}&   11,807.2 &     16,496.8 \\
         Road Runner &              18 &      200.0 &   6,878.0 &   35,215.0 &   43,156.0 &{\bf58,549.0}&   52,264.0 &     54,630.0 \\
            Robotank &              18 &        2.4 &       8.9 &       58.7 &       59.1 &{\bf62.0}&       56.2 &         24.7 \\
            Seaquest &              18 &      215.5 &  40,425.8 &    4,216.7 &   14,498.0 &{\bf37,361.6}&   25,463.7 &      1,431.2 \\
              Skiing &               3 &  -15,287.4 &  -3,686.6 &  -12,142.1 &  -11,490.4 &  -11,928.0 &{\bf-10,169.1}&    -18,955.8 \\
             Solaris &              18 &    2,047.2 &  11,032.6 &    1,295.4 &      810.0 &    1,768.4 &{\bf2,272.8}&        280.6 \\
      Space Invaders &               6 &      182.6 &   1,464.9 &    1,293.8 &    2,628.7 &    5,993.1 &    3,912.1 &{\bf8,978.0}\\
         Star Gunner &              18 &      697.0 &   9,528.0 &   52,970.0 &   58,365.0 &   90,804.0 &   61,582.0 &{\bf127,073.0}\\
           Surround  &               5 &       -9.7 &       5.4 &       -6.0 &        1.9 &        4.0 &{\bf5.9}&         -0.2 \\
              Tennis &              18 &      -21.4 &      -6.7 &{\bf11.1}&       -7.8 &        4.4 &       -5.3 &        -13.2 \\
          Time Pilot &              10 &    3,273.0 &   5,650.0 &    4,786.0 &{\bf6,608.0}&    6,601.0 &    5,963.0 &      4,871.0 \\
           Tutankham &               8 &       12.7 &     138.3 &       45.6 &       92.2 &       48.0 &       56.9 &{\bf108.6}\\
         Up and Down &               6 &      707.2 &   9,896.1 &    8,038.5 &   19,086.9 &{\bf24,759.2}&   12,157.4 &     22,681.3 \\
             Venture &              18 &       18.0 &   1,039.0 &      136.0 &       21.0 &{\bf200.0}&       94.0 &         29.0 \\
       Video Pinball &               9 &   20,452.0 &  15,641.1 &  154,414.1 &  367,823.7 &  110,976.2 &  295,972.8 &{\bf447,408.6}\\
       Wizard Of Wor &              10 &      804.0 &   4,556.0 &    1,609.0 &    6,201.0 &    7,054.0 &    5,727.0 &{\bf10,471.0}\\
       Yars' Revenge &              18 &    1,476.9 &  47,135.2 &    4,577.5 &    6,270.6 &   25,976.5 &    4,687.4 &{\bf58,145.9}\\
              Zaxxon &              18 &      475.0 &   8,443.0 &    4,412.0 &    8,593.0 &   10,164.0 &    9,474.0 &{\bf11,320.0}\\
  \end{tabular}
\end{center}
\end{table}

\begin{table}[!htb]
\caption{Normalized scores across all games. Starting with {\bf 30 no-op} actions.}
\footnotesize
\begin{center}
\begin{tabular}{l|rrr|rr}
       {\sc Games} &   {\sc DQN} &       {\sc DDQN} &       {\sc Duel} &{\sc Prior.} & {\sc Prior. Duel.} \\
\hline
               Alien &    20.2\% &    51.0\% &{\bf61.4\%}&    57.6\% &      53.8\% \\
              Amidar &    56.7\% &   104.3\% &{\bf137.1\%}&   107.0\% &     133.7\% \\
             Assault &   781.0\% &   995.1\% &   846.5\% &  1433.7\% &{\bf2166.0\%}\\
             Asterix &    50.0\% &   206.8\% &   337.4\% &   377.6\% &{\bf4520.1\%}\\
           Asteroids &     1.4\% &     0.0\% &{\bf4.5\%}&     4.1\% &       1.0\% \\
            Atlantis &  1651.2\% &   576.1\% &  2285.3\% &  2129.3\% &{\bf2366.9\%}\\
          Bank Heist &    59.7\% &   137.6\% &{\bf216.2\%}&   140.8\% &     201.5\% \\
         Battle Zone &    79.1\% &    84.2\% &{\bf99.9\%}&    83.8\% &      95.2\% \\
          Beam Rider &    49.9\% &    81.0\% &    71.2\% &   139.0\% &{\bf180.6\%}\\
             Berzerk &    18.4\% &    44.0\% &    53.8\% &    47.2\% &{\bf131.1\%}\\
             Bowling &    19.8\% &{\bf32.7\%}&    30.8\% &    18.0\% &      17.1\% \\
              Boxing &   732.5\% &   762.1\% &{\bf827.1\%}&   795.5\% &     823.1\% \\
            Breakout &  1334.5\% &{\bf1449.2\%}&  1194.5\% &  1294.3\% &    1266.6\% \\
           Centipede &    25.9\% &    33.4\% &    55.1\% &    23.9\% &{\bf56.4\%}\\
     Chopper Command &    80.8\% &    76.0\% &   158.2\% &   118.4\% &{\bf188.1\%}\\
       Crazy Climber &   399.1\% &   425.2\% &   530.1\% &   520.5\% &{\bf604.6\%}\\
            Defender &   131.3\% &   205.3\% &{\bf248.8\%}&   179.7\% &     243.1\% \\
        Demon Attack &   659.6\% &  3182.8\% &  3335.0\% &  3941.6\% &{\bf3998.3\%}\\
         Double Dunk &   557.7\% &   607.9\% &   866.5\% &{\bf1723.3\%}&     280.5\% \\
              Enduro &    84.7\% &   140.8\% &   262.4\% &   243.2\% &{\bf268.0\%}\\
       Fishing Derby &   163.8\% &   202.4\% &{\bf260.7\%}&   247.7\% &     251.1\% \\
             Freeway &   104.0\% &   112.5\% &     0.1\% &{\bf114.0\%}&     111.3\% \\
           Frostbite &    17.1\% &    37.9\% &   107.9\% &   101.1\% &{\bf172.1\%}\\
              Gopher &   395.4\% &   676.7\% &   717.5\% &  1495.6\% &{\bf4831.3\%}\\
            Gravitar &     9.4\% &     7.5\% &{\bf13.1\%}&    11.8\% &       2.0\% \\
            H.E.R.O. &    65.1\% &    64.1\% &    66.4\% &{\bf73.9\%}&      67.1\% \\
          Ice Hockey &    76.9\% &    70.0\% &    96.4\% &{\bf103.2\%}&      89.6\% \\
          James Bond &   270.1\% &   485.4\% &   468.8\% &{\bf1869.8\%}&     286.0\% \\
            Kangaroo &   241.6\% &   433.8\% &   496.2\% &{\bf541.3\%}&      58.3\% \\
               Krull &   639.3\% &   592.3\% &{\bf923.1\%}&   761.6\% &     822.2\% \\
      Kung-Fu Master &   114.8\% &   131.0\% &   151.4\% &   174.9\% &{\bf214.1\%}\\
 Montezuma's Revenge &{\bf0.0\%}&     0.0\% &     0.0\% &     0.0\% &       0.0\% \\
         Ms. Pac-Man &    41.8\% &    36.2\% &    89.9\% &{\bf93.5\%}&      45.5\% \\
      Name This Game &   102.8\% &   144.6\% &   168.1\% &   173.3\% &{\bf230.7\%}\\
             Phoenix &   119.2\% &   177.3\% &   344.5\% &   281.3\% &{\bf1073.3\%}\\
            Pitfall! &    -0.8\% &     3.0\% &{\bf3.4\%}&    -1.9\% &       3.4\% \\
                Pong &   114.0\% &   117.8\% &{\bf118.2\%}&   117.1\% &     118.0\% \\
         Private Eye &     0.2\% &     0.2\% &     0.1\% &{\bf0.3\%}&       0.3\% \\
              Q*Bert &    97.5\% &   112.3\% &{\bf143.4\%}&   121.1\% &     139.9\% \\
          River Raid &    38.3\% &    85.8\% &{\bf125.6\%}&    83.6\% &     122.1\% \\
         Road Runner &   504.7\% &   563.2\% &{\bf887.4\%}&   735.3\% &     793.3\% \\
            Robotank &   631.5\% &   643.7\% &{\bf645.1\%}&   617.5\% &     259.5\% \\
            Seaquest &    13.8\% &    39.0\% &{\bf119.5\%}&    62.6\% &       2.1\% \\
              Skiing &    31.6\% &    63.3\% &{\bf64.6\%}&    55.6\% &     -22.3\% \\
             Solaris &    20.3\% &    16.5\% &     9.1\% &{\bf27.7\%}&      -9.9\% \\
      Space Invaders &   101.6\% &   156.3\% &   412.9\% &   178.7\% &{\bf997.2\%}\\
         Star Gunner &   559.3\% &   620.5\% &   924.0\% &   653.4\% &{\bf1298.3\%}\\
           Surround  &    26.5\% &    43.2\% &    86.9\% &{\bf114.6\%}&      67.6\% \\
              Tennis &{\bf231.3\%}&     6.8\% &   186.2\% &   153.2\% &     153.2\% \\
          Time Pilot &    78.4\% &   287.2\% &{\bf487.5\%}&   338.9\% &     239.9\% \\
           Tutankham &    36.3\% &   132.5\% &   128.1\% &   123.7\% &{\bf150.1\%}\\
         Up and Down &    84.7\% &   201.1\% &{\bf397.9\%}&   140.0\% &     298.8\% \\
             Venture &    13.7\% &     8.3\% &{\bf41.9\%}&     4.5\% &       4.0\% \\
       Video Pinball &  1113.7\% &  1754.3\% &   555.9\% &  1596.2\% &{\bf2712.2\%}\\
       Wizard Of Wor &    51.0\% &   165.2\% &   173.9\% &   101.1\% &{\bf281.1\%}\\
       Yars' Revenge &    29.1\% &    16.7\% &    90.4\% &    16.1\% &{\bf129.2\%}\\
              Zaxxon &    58.3\% &   110.8\% &   141.3\% &   114.2\% &{\bf151.6\%}\\
\end{tabular}
\end{center}
\end{table}

\begin{table}[t]
\caption{Normalized scores across all games. Starting with {\bf Human Starts}.}
\footnotesize
\begin{center}
\begin{tabular}{l|rrr|rr}
              {\sc Games} &   {\sc DQN} &       {\sc DDQN} &       {\sc Duel} &{\sc Prior.} & {\sc Prior. Duel.} \\
\hline 
               Alien &     8.1\% &    14.5\% &{\bf21.8\%}&    19.3\% &      11.1\% \\
              Amidar &    10.9\% &    10.3\% &    10.5\% &     7.7\% &{\bf14.8\%}\\
             Assault &   719.2\% &  1275.9\% &   828.6\% &  1381.5\% &{\bf2334.4\%}\\
             Asterix &    40.8\% &   226.2\% &   212.7\% &   302.8\% &{\bf4938.4\%}\\
           Asteroids &     1.6\% &     0.9\% &{\bf3.3\%}&     2.5\% &       0.4\% \\
            Atlantis &  2128.0\% &  2335.5\% &{\bf3293.9\%}&  2419.0\% &    3125.3\% \\
          Bank Heist &    46.7\% &   138.8\% &{\bf177.8\%}&   137.3\% &     157.8\% \\
         Battle Zone &    68.5\% &    71.9\% &{\bf94.2\%}&    74.5\% &      91.9\% \\
          Beam Rider &    64.5\% &   116.7\% &    97.5\% &   210.3\% &{\bf252.7\%}\\
             Berzerk &    14.6\% &    39.9\% &    35.0\% &    32.8\% &{\bf97.1\%}\\
             Bowling &    19.2\% &{\bf30.9\%}&    27.5\% &    15.1\% &      13.7\% \\
              Boxing &   648.2\% &   677.0\% &   711.2\% &   666.7\% &{\bf728.5\%}\\
            Breakout &  1341.9\% &  1396.7\% &{\bf1559.0\%}&  1298.3\% &    1342.4\% \\
           Centipede &    24.4\% &    23.0\% &    35.2\% &    18.6\% &{\bf43.4\%}\\
     Chopper Command &    52.8\% &    34.4\% &    37.9\% &    48.2\% &{\bf89.5\%}\\
       Crazy Climber &   380.6\% &   447.7\% &   493.9\% &   506.5\% &{\bf508.0\%}\\
            Defender &   113.2\% &   207.2\% &   259.8\% &   176.0\% &{\bf263.2\%}\\
        Demon Attack &   381.6\% &  2151.6\% &  1734.8\% &  1888.0\% &{\bf2261.9\%}\\
         Double Dunk &   622.5\% &   982.5\% &   948.7\% &{\bf1998.7\%}&     328.7\% \\
              Enduro &    86.2\% &   158.0\% &   262.7\% &   232.7\% &{\bf280.5\%}\\
       Fishing Derby &    91.8\% &    97.7\% &    88.8\% &   105.7\% &{\bf114.5\%}\\
             Freeway &   105.1\% &   112.5\% &     0.6\% &{\bf113.1\%}&     110.2\% \\
           Frostbite &    10.4\% &    33.4\% &    54.8\% &    83.2\% &{\bf96.0\%}\\
              Gopher &   385.3\% &   727.9\% &   960.8\% &  1679.2\% &{\bf5089.7\%}\\
            Gravitar &{\bf1.8\%}&    -1.6\% &     1.8\% &     0.8\% &      -2.7\% \\
            H.E.R.O. &    55.3\% &    54.9\% &    56.2\% &{\bf79.6\%}&      57.2\% \\
          Ice Hockey &    79.2\% &    70.8\% &    82.4\% &    92.5\% &{\bf99.4\%}\\
          James Bond &   198.2\% &   161.0\% &   239.4\% &{\bf1172.4\%}&     164.6\% \\
            Kangaroo &   166.6\% &   420.8\% &   387.8\% &{\bf457.9\%}&      28.8\% \\
               Krull &   528.0\% &   589.7\% &{\bf720.8\%}&   597.7\% &     679.8\% \\
      Kung-Fu Master &   100.5\% &   146.0\% &   117.1\% &   153.2\% &{\bf181.5\%}\\
 Montezuma's Revenge &     0.5\% &     0.4\% &    -0.1\% &{\bf0.6\%}&      -0.0\% \\
         Ms. Pac-Man &     5.9\% &     6.9\% &{\bf13.5\%}&    11.0\% &       5.3\% \\
      Name This Game &    98.9\% &   142.9\% &   186.9\% &   173.3\% &{\bf235.5\%}\\
             Phoenix &   114.4\% &   202.3\% &   347.2\% &   284.0\% &{\bf1125.1\%}\\
            Pitfall! &     3.7\% &     2.6\% &{\bf4.8\%}&    -1.2\% &       1.7\% \\
                Pong &   107.6\% &{\bf110.9\%}&   110.0\% &   110.1\% &     108.6\% \\
         Private Eye &    -0.7\% &    -1.9\% &    -0.6\% &     0.0\% &{\bf1.0\%}\\
              Q*Bert &    76.4\% &    91.1\% &{\bf117.6\%}&    82.0\% &     116.6\% \\
          River Raid &    30.2\% &    74.3\% &{\bf115.9\%}&    81.3\% &     115.3\% \\
         Road Runner &   524.3\% &   643.2\% &{\bf873.7\%}&   779.6\% &     815.1\% \\
            Robotank &   863.3\% &   868.7\% &{\bf913.3\%}&   824.4\% &     341.1\% \\
            Seaquest &    10.0\% &    35.5\% &{\bf92.4\%}&    62.8\% &       3.0\% \\
              Skiing &    27.1\% &    32.7\% &    29.0\% &{\bf44.1\%}&     -31.6\% \\
             Solaris &    -8.4\% &   -13.8\% &    -3.1\% &{\bf2.5\%}&     -19.7\% \\
      Space Invaders &    86.7\% &   190.8\% &   453.1\% &   290.8\% &{\bf685.9\%}\\
         Star Gunner &   591.9\% &   653.0\% &  1020.3\% &   689.4\% &{\bf1431.0\%}\\
           Surround  &    24.7\% &    76.9\% &    91.1\% &{\bf103.2\%}&      62.9\% \\
              Tennis &{\bf220.8\%}&    92.1\% &   175.0\% &   109.6\% &      55.6\% \\
          Time Pilot &    63.7\% &{\bf140.3\%}&   140.0\% &   113.2\% &      67.2\% \\
           Tutankham &    26.2\% &    63.3\% &    28.1\% &    35.2\% &{\bf76.4\%}\\
         Up and Down &    79.8\% &   200.0\% &{\bf261.8\%}&   124.6\% &     239.1\% \\
             Venture &    11.6\% &     0.3\% &{\bf17.8\%}&     7.4\% &       1.1\% \\
       Video Pinball &   987.2\% &  2351.6\% &   709.5\% &  1892.3\% &{\bf2860.5\%}\\
       Wizard Of Wor &    21.5\% &   143.8\% &   166.6\% &   131.2\% &{\bf257.6\%}\\
       Yars' Revenge &     6.8\% &    10.5\% &    53.7\% &     7.0\% &{\bf124.1\%}\\
              Zaxxon &    49.4\% &   101.9\% &   121.6\% &   112.9\% &{\bf136.1\%}\\
            \hline
            {\bf Mean}   &    219.6\% & 332.9\% &  343.8\% & 386.7\% & {\bf 567.0}\%\\
            {\bf Median}   &68.5\% & 110.9\% & {\bf117.1}\% & 112.9\% & 115.3\%\\
\end{tabular}
\end{center}
\end{table}
