# Supplementary material for: Dueling Network Architectures for Deep Reinforcement Learning
Source: arXiv:1511.06581 source file (2016-04-05)
Supplement: Supplementary file 2 [file ddqn_appendix.tex]

%!TEX root = main.tex
\begin{algorithm2e}[h!]
\small
\SetKwInOut{Input}{input}\SetKwInOut{Output}{output}
\Input{$\mathcal{D}$ -- empty replay buffer; $\theta$ -- initial network parameters, $\theta^-$ -- copy of $\theta$}
\Input{$N_r$ -- replay buffer maximum size; $N_b$ -- training batch size; $N^-$ -- target network replacement freq.}
\For{\mbox{episode} $e \in \{ 1, 2, \ldots, M$ \} } {
  Initialize frame sequence $\mathbf{x} \leftarrow ()$ \;
  \For{$t \in \{ 0, 1, \ldots \} $} {
    Set state $s \leftarrow \mathbf{x}$, sample action $a \sim \pi_\mathcal{B}$ \;
    Sample next frame $x^t$ from environment $\mathcal{E}$ given $(s,a)$ and receive reward $r$, and append $x^t$ to $\mathbf{x}$ \;
    {\bf if} {$|\mathbf{x}| > N_f$} {\bf then} delete oldest frame $x_{t_{min}}$ from $\mathbf{x}$ {\bf end} \;
    Set $s' \leftarrow \mathbf{x}$, and add transition tuple $(s, a, r, s')$ to $\mathcal{D}$,\\~~~~~~~~~replacing the oldest tuple if $|\mathcal{D}| \ge N_r$ \;
    Sample a minibatch of $N_b$ tuples $(s, a, r, s') \sim \mbox{Unif}(\mathcal{D})$\; %uniformly from $\mathcal{D}$ \;
    Construct target values, one for each of the $N_b$ tuples: \;
    Define $a^{\max{}}(s'; \theta) = \argmax_{a'} Q(s', a'; \theta)$\;
    $y_j = \left\{ \begin{array}{ll}
         r & \mbox{if $s'$ is terminal}\\
         r + \gamma Q(s', a^{\max{}}(s'; \theta); \theta^-), & \mbox{otherwise}. \end{array} \right.$ \;
    Do a gradient descent step with loss $\|y_j - Q(s, a ; \theta )\|^2$ \;
    Replace target parameters $\theta^- \leftarrow \theta$ every $N^-$ steps\;
  }
}
\caption{Double DQN Algorithm.}\label{alg:ddqn}
\end{algorithm2e}
