# Supplementary material for: Dueling Network Architectures for Deep Reinforcement Learning
Source: arXiv:1511.06581 source file (2016-04-05)
Supplement: Supplementary file 3 [file small_appendix.tex]

%!TEX root = main.tex
\label{sec:appen}

\begin{table}[h!]
\vspace{-0.25cm}
\caption{Normalized scores, starting with {\bf 30 no-op} actions.}
\footnotesize
\begin{center}
\begin{tabular}{l|rrr}

              Games &      DQN &     DDQN &     Duel \\
              \hline 
               Alien &    20.2\% &    51.0\% &{\bf61.4\%}\\
              Amidar &    56.7\% &   104.3\% &{\bf137.1\%}\\
             Assault &   781.0\% &{\bf995.1\%}&   846.5\% \\
             Asterix &    50.0\% &   206.8\% &{\bf337.4\%}\\
           Asteroids &     1.4\% &     0.0\% &{\bf4.5\%}\\
            Atlantis &  1651.2\% &   576.1\% &{\bf2285.3\%}\\
          Bank Heist &    59.7\% &   137.6\% &{\bf216.2\%}\\
         Battle Zone &    79.1\% &    84.2\% &{\bf99.9\%}\\
          Beam Rider &    49.9\% &{\bf81.0\%}&    71.2\% \\
             Berzerk &    18.4\% &    44.0\% &{\bf53.8\%}\\
             Bowling &    19.8\% &{\bf32.7\%}&    30.8\% \\
              Boxing &   732.5\% &   762.1\% &{\bf827.1\%}\\
            Breakout &  1334.5\% &{\bf1449.2\%}&  1194.5\% \\
           Centipede &    25.9\% &    33.4\% &{\bf55.1\%}\\
     Chopper Command &    80.8\% &    76.0\% &{\bf158.2\%}\\
       Crazy Climber &   399.1\% &   425.2\% &{\bf530.1\%}\\
            Defender &   131.3\% &   205.3\% &{\bf248.8\%}\\
        Demon Attack &   659.6\% &  3182.8\% &{\bf3335.0\%}\\
         Double Dunk &   557.7\% &   607.9\% &{\bf866.5\%}\\
              Enduro &    84.7\% &   140.8\% &{\bf262.4\%}\\
       Fishing Derby &   163.8\% &   202.4\% &{\bf260.7\%}\\
             Freeway &   104.0\% &{\bf112.5\%}&     0.1\% \\
           Frostbite &    17.1\% &    37.9\% &{\bf107.9\%}\\
              Gopher &   395.4\% &   676.7\% &{\bf717.5\%}\\
            Gravitar &     9.4\% &     7.5\% &{\bf13.1\%}\\
            H.E.R.O. &    65.1\% &    64.1\% &{\bf66.4\%}\\
          Ice Hockey &    76.9\% &    70.0\% &{\bf96.4\%}\\
          James Bond &   270.1\% &{\bf485.4\%}&   468.8\% \\
            Kangaroo &   241.6\% &   433.8\% &{\bf496.2\%}\\
               Krull &   639.3\% &   592.3\% &{\bf923.1\%}\\
      Kung-Fu Master &   114.8\% &   131.0\% &{\bf151.4\%}\\
 Montezuma's Revenge &{\bf0.0\%}&     0.0\% &     0.0\% \\
         Ms. Pac-Man &    41.8\% &    36.2\% &{\bf89.9\%}\\
      Name This Game &   102.8\% &   144.6\% &{\bf168.1\%}\\
             Phoenix &   119.2\% &   177.3\% &{\bf344.5\%}\\
            Pitfall! &    -0.8\% &     3.0\% &{\bf3.4\%}\\
                Pong &   114.0\% &   117.8\% &{\bf118.2\%}\\
         Private Eye &{\bf0.2\%}&     0.2\% &     0.1\% \\
              Q*Bert &    97.5\% &   112.3\% &{\bf143.4\%}\\
          River Raid &    38.3\% &    85.8\% &{\bf125.6\%}\\
         Road Runner &   504.7\% &   563.2\% &{\bf887.4\%}\\
            Robotank &   631.5\% &   643.7\% &{\bf645.1\%}\\
            Seaquest &    13.8\% &    39.0\% &{\bf119.5\%}\\
              Skiing &    31.6\% &    63.3\% &{\bf64.6\%}\\
             Solaris &{\bf20.3\%}&    16.5\% &     9.1\% \\
      Space Invaders &   101.6\% &   156.3\% &{\bf412.9\%}\\
         Star Gunner &   559.3\% &   620.5\% &{\bf924.0\%}\\
           Surround  &    26.5\% &    43.2\% &{\bf86.9\%}\\
              Tennis &{\bf231.3\%}&     6.8\% &   186.2\% \\
          Time Pilot &    78.4\% &   287.2\% &{\bf487.5\%}\\
           Tutankham &    36.3\% &{\bf132.5\%}&   128.1\% \\
         Up and Down &    84.7\% &   201.1\% &{\bf397.9\%}\\
             Venture &    13.7\% &     8.3\% &{\bf41.9\%}\\
       Video Pinball &  1113.7\% &{\bf1754.3\%}&   555.9\% \\
       Wizard Of Wor &    51.0\% &   165.2\% &{\bf173.9\%}\\
       Yars' Revenge &    29.1\% &    16.7\% &{\bf90.4\%}\\
              Zaxxon &    58.3\% &   110.8\% &{\bf141.3\%}\\
            \hline
            {\bf Mean}   &    227.9\% & 307.3\% &  {\bf373.1}\% \\
            {\bf Median}   &79.1\% & 117.8\% & {\bf151.4}\% \\
\end{tabular}
\end{center}
\end{table}
